# Supplementary material for: Training Deep SLAM on Single Frames
Source: arXiv:1912.05405 source file (2019-12-11)
Supplement: Supplementary file 1 [file arXiv_DeepSLAM_supplementary.pdf]

# Training Deep SLAM on Single Frames

## — Supplementary Material —

### 1. Optical flow synthesis

We provide several examples of synthesized and estimated optical flow (OF) for KITTI dataset on Figure 1 and for EuRoC dataset on Figure 2. It can be observed that estimated OF is more cluttered compared to synthesized OF, while synthesized OF is more smooth.

### 2. Detailed description of experiments

We present detailed comparison of our method with other deep learning-based monocular visual odometry and SLAM methods on KITTI. We report results on sequences 03, 04, 05, 06, 07, 10 (Figure 3) which are commonly used for evaluation. We train our network for 5 times and report the average values for translation error  $t_{err}$ , rotation error  $r_{err}$  and ATE. Since sequences 03, 04, 10 do not contain loops, the results of our visual odometry and SLAM models do not differ.

**Unsupervised methods.** Results for each of the sequences 03, 04, 05, 06, 07, 10 are shown in Table 3. Overall, our visual odometry outperforms listed unsupervised methods. It shows better results than SGANVO[3] on sequences 03 and 10 and performs at the same level on sequences 05 and 06. According to Table 3, adding graph optimization helps to improve results for trajectories with loops. Thus, we believe that our method of converting visual odometry model to SLAM system can be used along with standard unsupervised learning pipeline.

**Supervised methods.** We evaluate our visual odometry and SLAM against supervised methods on sequences 03, 04, 05, 06, 07, 10 from KITTI. The results are reported in Table 4. While our model is quite simple and accounts only for pairs of similar frames, it outperforms more complex models. This may indicate that not the choice of proper network architecture, but the lack of training data is the major difficulty when developing a trainable visual odometry method. Therefore, in our work we address this issue rather than focus on improving the network architecture.

**Pose graphs visualization.** Figure 5 shows the graphs that were used for optimization. Here blue edges correspond to consecutive frames and orange edges correspond to detected loops.

| 6DoF      | $NN_{cons}$    |                   | $NN_{loops}$   |                   |
|-----------|----------------|-------------------|----------------|-------------------|
|           | $\mu, 10^{-2}$ | $\sigma, 10^{-2}$ | $\mu, 10^{-2}$ | $\sigma, 10^{-2}$ |
| $x$       | -0.01          | 2.64              | 1.54           | 20.31             |
| $y$       | -1.72          | 1.88              | -3.41          | 32                |
| $z$       | 92.19          | 29.77             | 139.6          | 131               |
| $euler_x$ | 0              | 0.3               | 0.03           | 0.62              |
| $euler_y$ | 0.07           | 1.83              | 0.28           | 6.39              |
| $euler_z$ | 0              | 0.28              | 0.01           | 0.63              |

Table 1: Parameters of t-distributions with  $\nu = 4$  degrees of freedom that were used to approximate motions on KITTI dataset.  $\mu$  and  $\sigma$  for  $x, y, z$  are in meters and for  $euler_x, euler_y, euler_z$  are in radians

| 6DoF      | $NN_{cons}$    |                   | $NN_{loops}$   |                   |
|-----------|----------------|-------------------|----------------|-------------------|
|           | $\mu, 10^{-3}$ | $\sigma, 10^{-2}$ | $\mu, 10^{-3}$ | $\sigma, 10^{-2}$ |
| $x$       | 4.2            | 2.6               | 17.8           | 12.8              |
| $y$       | -3.26          | 5.56              | 17.2           | 21.6              |
| $z$       | 8.49           | 3.26              | 50             | 29.2              |
| $euler_x$ | -1.03          | 2.26              | -1.9           | 12                |
| $euler_y$ | 0.354          | 1.77              | 0.69           | 3.9               |
| $euler_z$ | 0.391          | 1.54              | -1.6           | 5.4               |

Table 2: Parameters of t-distributions with  $\nu = 4$  degrees of freedom that were used to approximate motions on EuRoC dataset.  $\mu$  and  $\sigma$  for  $x, y, z$  are in meters and for  $euler_x, euler_y, euler_z$  are in radians

### 3. Additional ablation studies

**Error analysis for monocular visual odometry.** To analyse distribution of the errors of supervised visual odometry we plot the values of error with respect to the distance traveled. These plots are showed in Figure 6. We show errors for consecutive frames (with  $NN_{cons}$ ) and for loops (with  $NN_{loops}$ ). One can notice that the errors of the  $NN_{loops}$  are significantly larger than the errors for consecutive frames, and overall the larger is the magnitude of the motion, the larger is the error.

<sup>2</sup>the updated model in Github is evaluated

<sup>2</sup>currently the top monocular method on KITTI test

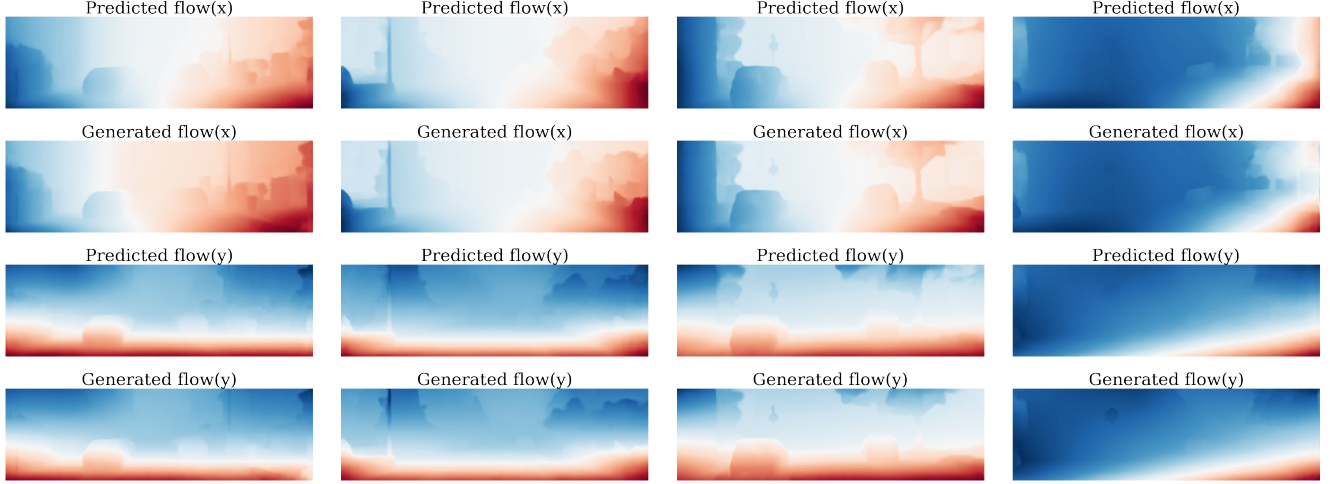

Figure 1: Examples of predicted optical flow with PWC-net[6] and synthesised optical flow for KITTI dataset

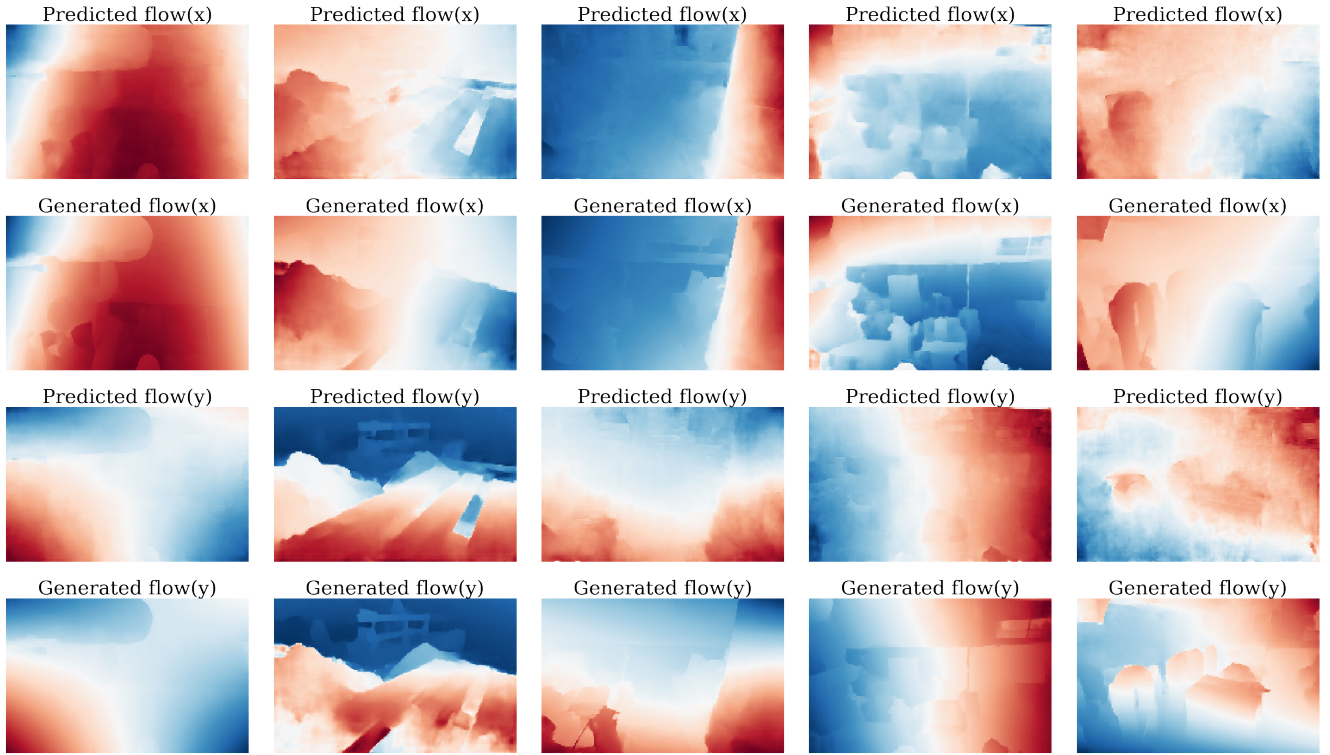

Figure 2: Examples of predicted optical flow with PWC-net[6] and synthesised optical flow for EuRoC dataset

**Analysis of motion distribution.** We analyse the joint distributions for all pairs of motion components between consecutive frames on KITTI and EuRoC datasets in Figure 7 and Figure 8 respectively. Figures show the 2d distribution plots. We approximate 6DoF with 6 independent t-distributions. Estimated parameters for these distributions are listed in Table 1 for KITTI dataset and in Table 2 for EuRoC dataset. We also plot the motions sampled from the

t-distribution used in our experiments. It can be seen that in most cases the synthetic samples and real samples appear in very similar locations.

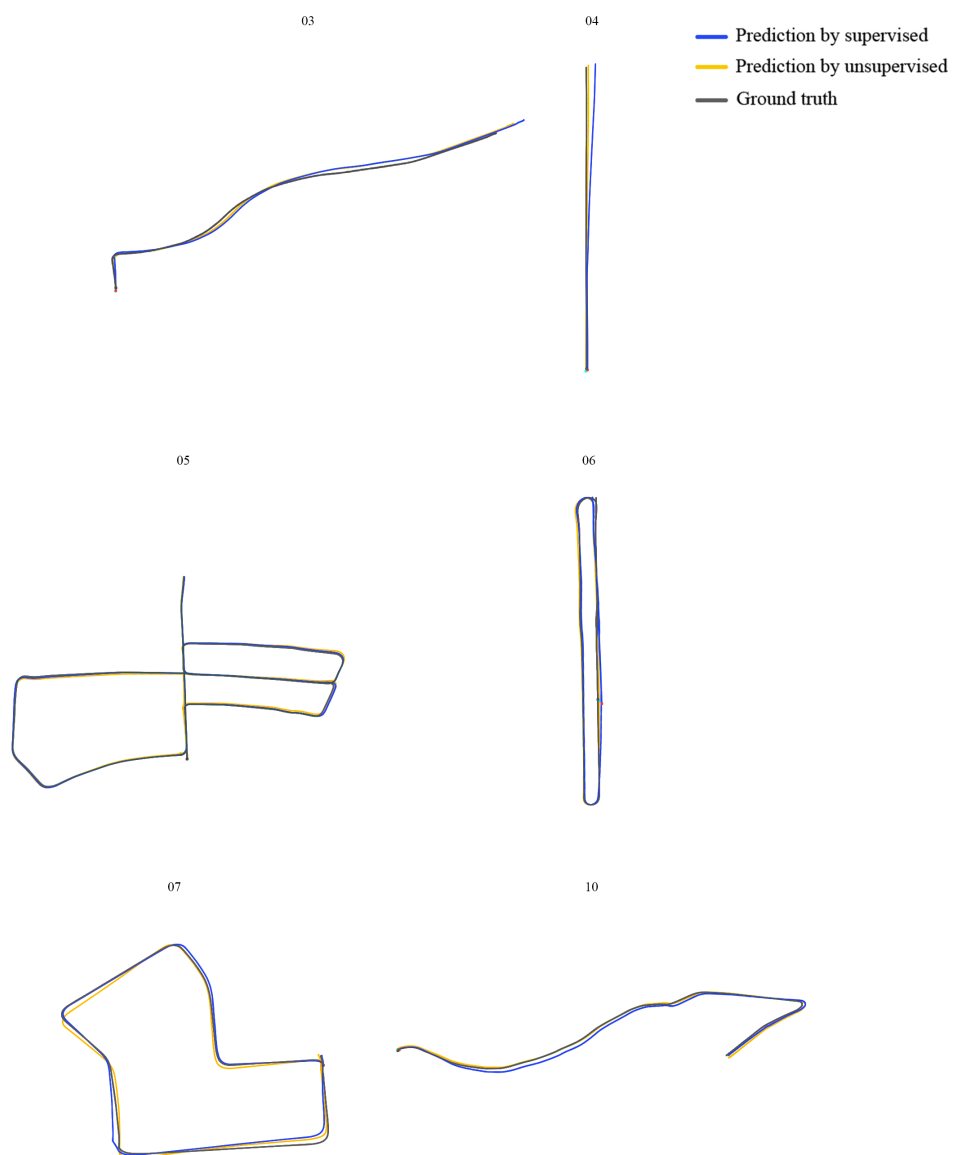

Figure 3: 03, 04, 05, 06, 07, 10 sequences of KITTI dataset predicted by our supervised and unsupervised SLAM models.

| Method                      | Metric    | 03          | 04          | 05          | 06          | 07          | 10          | Avg         |
|-----------------------------|-----------|-------------|-------------|-------------|-------------|-------------|-------------|-------------|
| SfMLearner[14] <sup>1</sup> | $t_{err}$ | 12.56       | 4.32        | 12.99       | 15.55       | 12.61       | 15.25       | 12.21       |
|                             | $r_{err}$ | <u>4.52</u> | 3.28        | 4.66        | 5.58        | 6.31        | 4.06        | 4.74        |
|                             | $ATE$     | 8.42        | 3.10        | 60.89       | 52.19       | 20.12       | 24.09       | 28.14       |
| Depth-VO-Feat[12]           | $t_{err}$ | 15.76       | 3.14        | 4.94        | 5.80        | 6.49        | 12.82       | 8.15        |
|                             | $r_{err}$ | 10.62       | 2.02        | 2.34        | 2.06        | 3.56        | 3.41        | 4.00        |
|                             | $ATE$     | 21.34       | 3.12        | 22.15       | 14.31       | 15.35       | 24.70       | 16.83       |
| SC-SfMLearner[1]            | $t_{err}$ | 9.22        | 4.22        | 6.70        | 5.36        | 8.29        | 10.74       | 7.42        |
|                             | $r_{err}$ | 4.93        | 2.01        | 2.38        | 1.65        | 4.53        | 4.58        | 3.35        |
|                             | $ATE$     | 10.21       | 2.97        | 40.56       | 12.56       | 21.01       | 20.19       | 17.92       |
| UnDeepVO[4]                 | $t_{err}$ | <u>5.00</u> | 5.49        | 3.40        | 6.20        | 3.15        | 10.63       | 5.65        |
|                             | $r_{err}$ | 6.17        | 2.13        | 1.50        | 1.98        | 2.48        | 4.65        | 3.15        |
| GeoNet[11]                  | $t_{err}$ | 19.21       | 9.09        | 20.12       | 9.28        | 8.27        | 20.73       | 13.12       |
|                             | $r_{err}$ | 9.78        | 7.54        | 7.67        | 4.34        | 5.93        | 9.04        | 7.38        |
| Vid2Depth[5]                | $t_{err}$ | 27.12       | 18.92       | 51.13       | 58.07       | 51.22       | 21.54       | 37.98       |
|                             | $r_{err}$ | 10.39       | 1.19        | 21.86       | 26.83       | 36.64       | 12.54       | 18.24       |
| SGANVO[3] <sup>2</sup>      | $t_{err}$ | 10.56       | <b>2.40</b> | 3.25        | <b>3.99</b> | <b>4.67</b> | 5.89        | <u>5.12</u> |
|                             | $r_{err}$ | 6.30        | <b>0.77</b> | 1.31        | 1.46        | <b>1.83</b> | 3.56        | 2.53        |
| Ours (unsup) VO             | $t_{err}$ | <b>2.98</b> | 12.70       | 4.64        | 5.81        | 13.28       | <b>3.99</b> | 5.57        |
|                             | $r_{err}$ | <b>0.93</b> | 1.72        | 1.68        | 1.68        | 8.76        | <b>1.13</b> | <u>2.23</u> |
|                             | $ATE$     | 1.08        | 2.08        | 18.53       | 14.25       | 4.64        | 5.20        | 14.30       |
| Ours (unsup) SLAM           | $t_{err}$ | <b>2.98</b> | 12.70       | <b>2.15</b> | 4.07        | 7.24        | <b>3.99</b> | <b>3.37</b> |
|                             | $r_{err}$ | <b>0.93</b> | 1.72        | <b>0.81</b> | <b>0.86</b> | 4.41        | <b>1.13</b> | <b>1.24</b> |
|                             | $ATE$     | 1.08        | 2.08        | 2.62        | 3.69        | 5.18        | 5.20        | <b>3.24</b> |

Table 3: Results of unsupervised deep learning-based methods on test trajectories from KITTI dataset. The best results are shown in bold. The second best is underlined.

| Method                      | Metric    | 03          | 04          | 05          | 06          | 07          | 10          | Avg         |
|-----------------------------|-----------|-------------|-------------|-------------|-------------|-------------|-------------|-------------|
| 2D-Flow[13]                 | $t_{err}$ | 3.35        | 4.15        | 2.49        | 3.19        | 17.20       | 7.24        | 6.27        |
|                             | $r_{err}$ | 1.62        | 2.53        | 1.19        | 1.54        | 10.40       | 3.06        | 3.39        |
| 3D-Flow[13]                 | $t_{err}$ | <b>3.18</b> | 2.04        | 2.59        | 1.39        | 2.81        | 4.38        | 2.73        |
|                             | $r_{err}$ | <b>1.31</b> | 0.81        | 0.99        | 0.95        | 2.54        | 3.12        | 1.62        |
| DeepVO[7]                   | $t_{err}$ | 8.49        | 7.19        | 2.62        | 5.42        | 3.91        | 8.11        | 5.96        |
|                             | $r_{err}$ | 6.89        | 6.97        | 3.61        | 5.82        | 4.60        | 8.83        | 6.12        |
| ESP-VO[8]                   | $t_{err}$ | 6.72        | 6.33        | 3.35        | 7.24        | 3.52        | 9.77        | 6.15        |
|                             | $r_{err}$ | 6.46        | 6.08        | 4.93        | 7.29        | 5.02        | 10.20       | 6.63        |
| SRNN <sub>channel</sub> [9] | $t_{err}$ | 5.44        | 2.91        | 3.27        | 8.50        | 3.37        | 6.32        | 4.80        |
|                             | $r_{err}$ | 3.32        | 1.30        | 1.62        | 2.74        | 2.25        | 2.33        | 2.26        |
| LS-VO[2]                    | $t_{err}$ | 5.30        | <b>0.78</b> | 2.36        | 2.91        | 3.51        | 3.31        | 2.54        |
|                             | $r_{err}$ | 1.53        | <b>0.42</b> | 0.91        | 1.14        | 5.53        | 1.26        | 1.80        |
| SMRP[10]                    | $t_{err}$ | 3.32        | 2.96        | 2.59        | 4.93        | <b>3.07</b> | 3.94        | 3.47        |
|                             | $r_{err}$ | 2.10        | 1.76        | 1.25        | 1.90        | <b>1.76</b> | 1.72        | 1.75        |
| Ours (sup) VO               | $t_{err}$ | 4.23        | 4.42        | 1.43        | 1.97        | 4.48        | <b>2.01</b> | <u>2.07</u> |
|                             | $r_{err}$ | 1.70        | 1.08        | 0.60        | 0.77        | 2.89        | <b>0.74</b> | <u>0.93</u> |
|                             | $ATE$     | 1.57        | 1.01        | 5.53        | 7.21        | 7.35        | 2.53        | <u>4.38</u> |
| Ours (sup) SLAM             | $t_{err}$ | 4.23        | 4.42        | <b>0.86</b> | <b>1.05</b> | 3.58        | <b>2.01</b> | <b>1.54</b> |
|                             | $r_{err}$ | 1.70        | 1.08        | <b>0.38</b> | <b>0.44</b> | 2.49        | <b>0.74</b> | <b>0.74</b> |
|                             | $ATE$     | 1.57        | 1.01        | 1.52        | 1.33        | 3.36        | 2.53        | <b>1.84</b> |

Table 4: Results of supervised deep-learning-based methods on test trajectories from KITTI dataset. The best results are shown in bold. The second best is underlined.

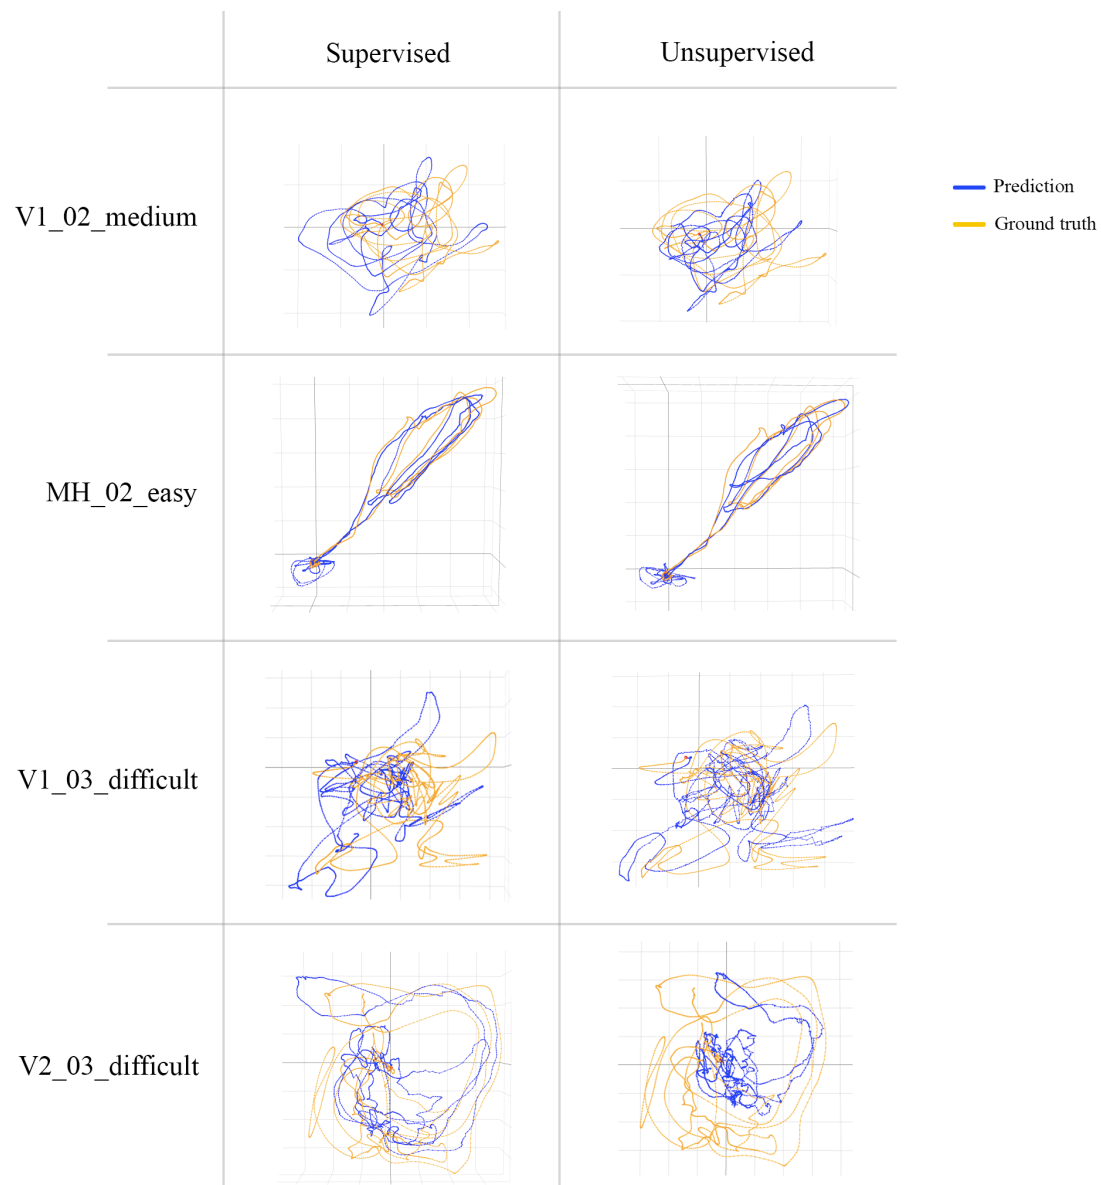

Figure 4: Predicted trajectories for V1\_02\_medium, MH\_02\_easy, V1\_03\_difficult, V2\_03\_difficult sequences of EuRoC dataset by our supervised and unsupervised SLAM models.

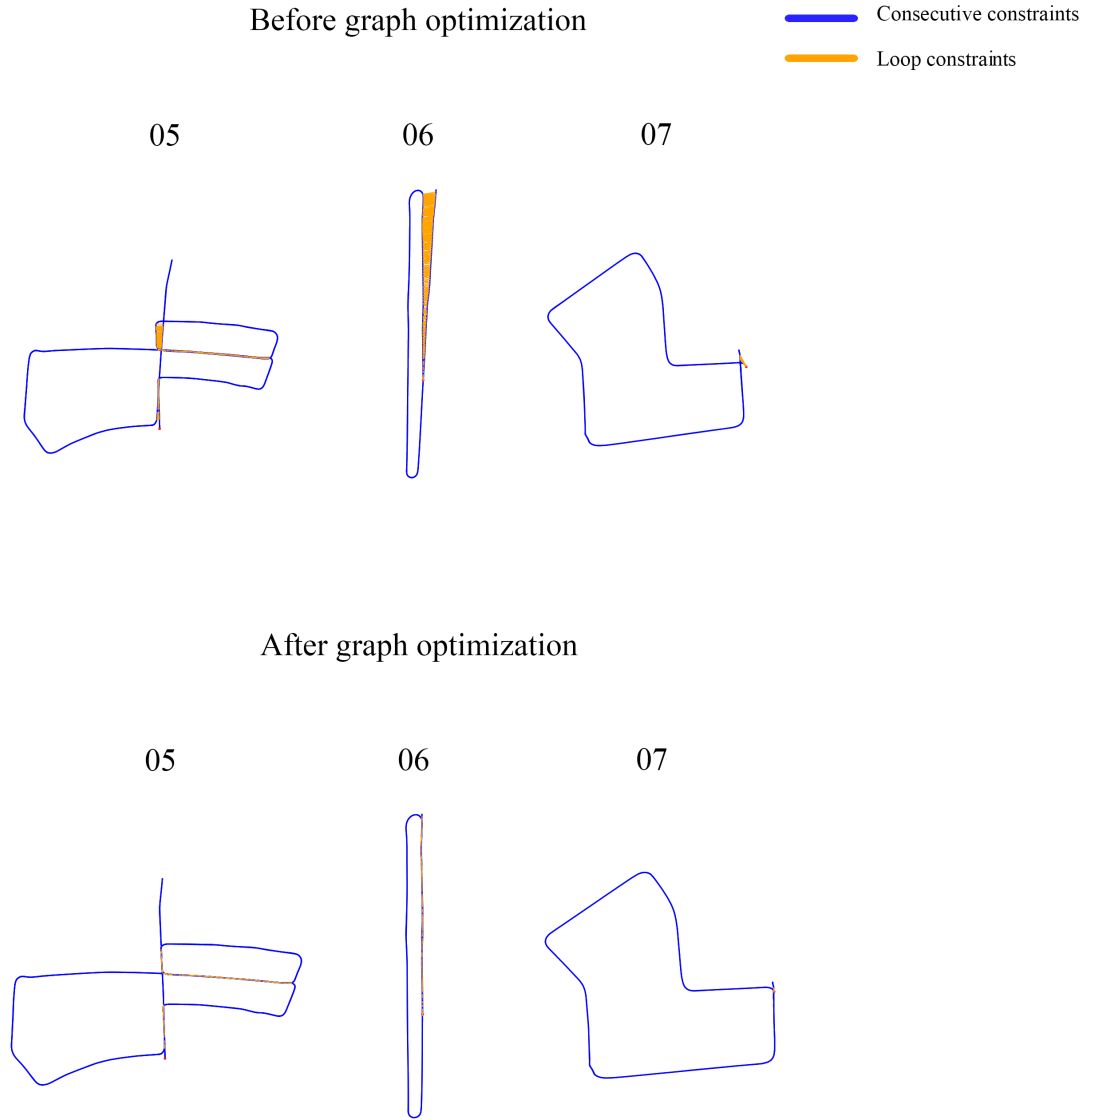

Figure 5: Pose graphs for trajectories from KITTI. The edges connect either consecutive frames or the pairs of frames where loop closure was detected. The first type of links in a graph is shown in blue. The second type of links is shown in orange.

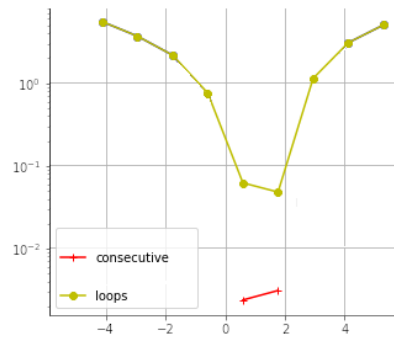

Figure 6: Errors of supervised visual odometry with respect to magnitude of the motion on KITTI dataset.

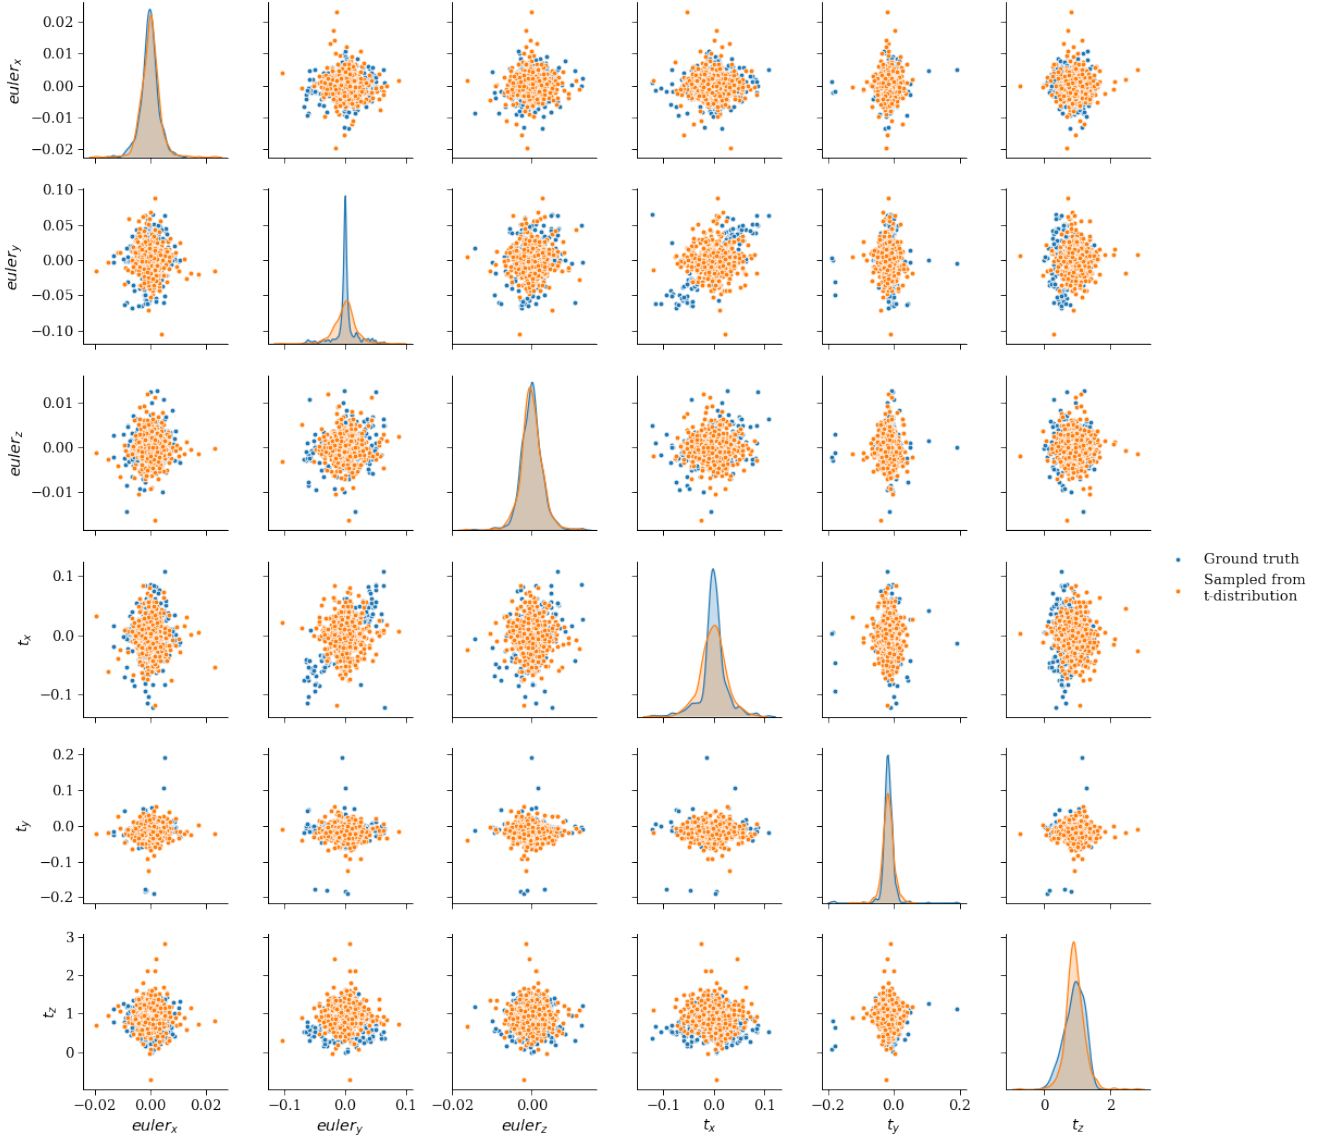

Figure 7: Motion distributions for training  $NN_{cons}$  on KITTI dataset. The subplots show pairwise joint distributions for all pairs of the motion components (Euler angles  $x$ ,  $y$ ,  $z$  and translations  $x$ ,  $y$ ,  $z$ ). Blue dots are real samples and orange dots are synthetic samples.

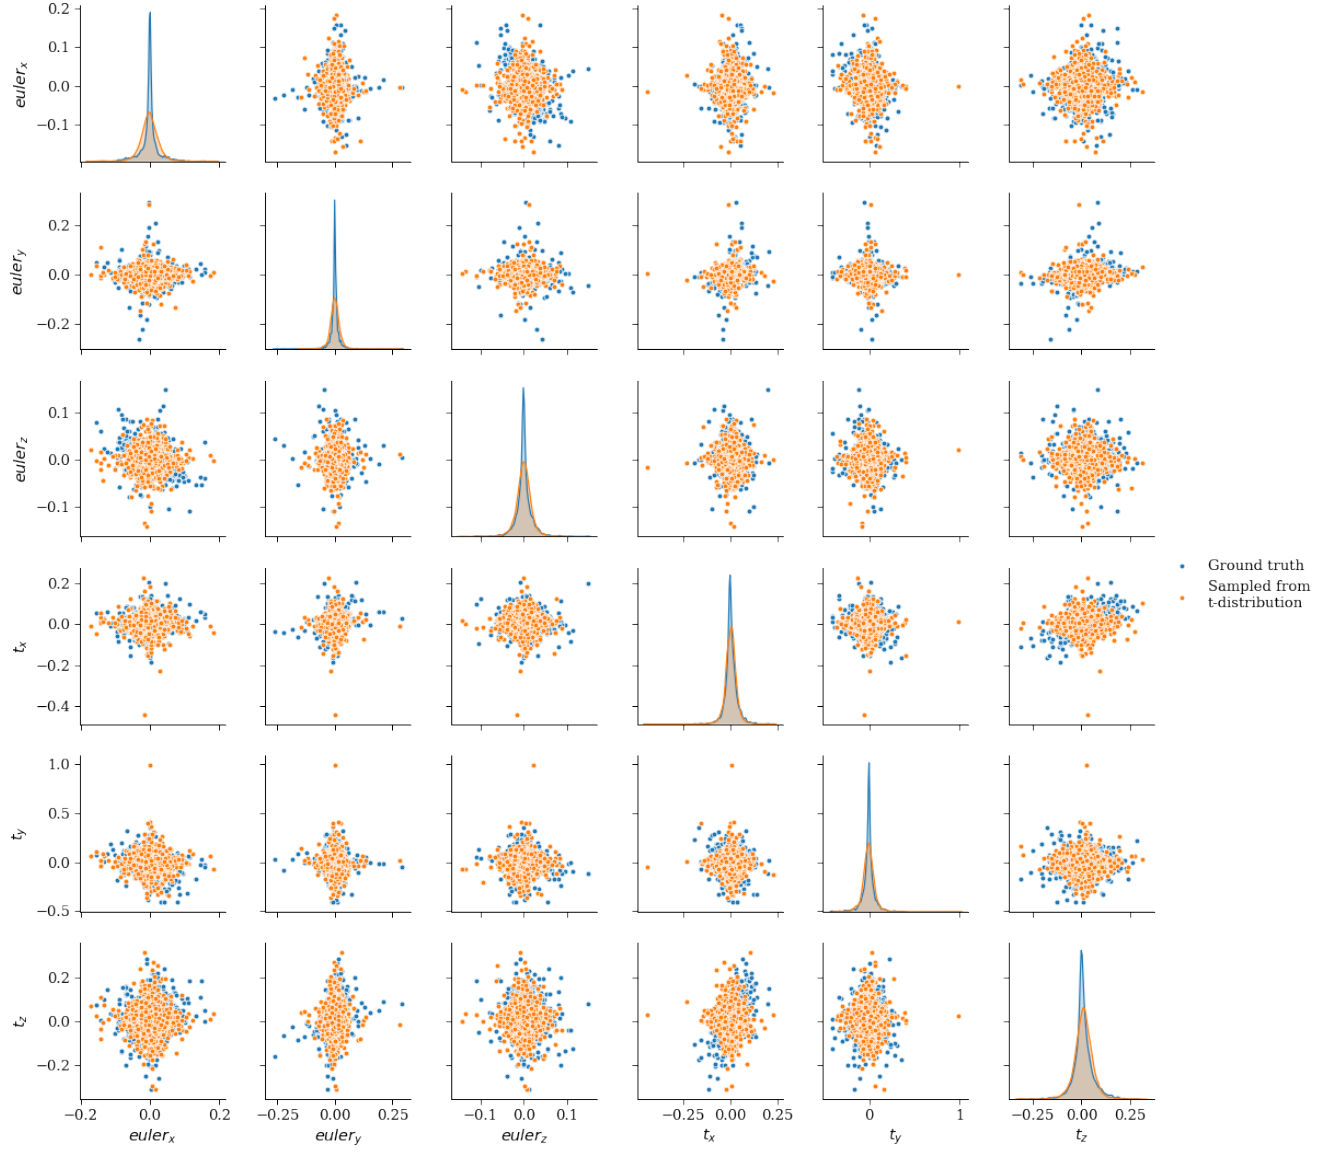

Figure 8: Motion distributions for training  $NN_{cons}$  on EuRoC dataset. The subplots show pairwise joint distributions for all pairs of the motion components (Euler angles  $x$ ,  $y$ ,  $z$  and translations  $x$ ,  $y$ ,  $z$ ). Blue dots are real samples and orange dots are synthetic samples.

## References

- [1] J.-W. Bian, Z. Li, N. Wang, H. Zhan, C. Shen, M.-M. Cheng, and R. I. Unsupervised scale-consistent depth and ego-motion learning from monocular video. *arXiv preprint arXiv:1908.10553*, 2019. 4
- [2] G. Costante and T. A. Ciarfuglia. LS-VO: learning dense optical subspace for robust visual odometry estimation. *CoRR*, abs/1709.06019, 2017. 4
- [3] T. Feng and D. Gu. SGANVO: unsupervised deep visual odometry and depth estimation with stacked generative adversarial networks. *CoRR*, abs/1906.08889, 2019. 1, 4
- [4] R. Li, S. Wang, Z. Long, and D. Gu. Undeepvo: Monocular visual odometry through unsupervised deep learning. *CoRR*, abs/1709.06841, 2017. 4
- [5] R. Mahjourian, M. Wicke, and A. Angelova. Unsupervised learning of depth and ego-motion from monocular video using 3d geometric constraints. In *Proceedings of the IEEE Conference on Computer Vision and Pattern Recognition*, pages 5667–5675, 2018. 4
- [6] D. Sun, X. Yang, M.-Y. Liu, and J. Kautz. Pwc-net: Cnns for optical flow using pyramid, warping, and cost volume. In *Proceedings of the IEEE Conference on Computer Vision and Pattern Recognition*, pages 8934–8943, 2018. 2
- [7] S. Wang, R. Clark, H. Wen, and N. Trigoni. Deepvo: Towards end-to-end visual odometry with deep recurrent convolutional neural networks. In *Robotics and Automation (ICRA), 2017 IEEE International Conference on*, pages 2043–2050. IEEE, 2017. 4
- [8] S. Wang, R. Clark, H. Wen, and N. Trigoni. End-to-end, sequence-to-sequence probabilistic visual odometry through deep neural networks. *The International Journal of Robotics Research*, 37(4-5):513–542, 2018. 4
- [9] F. Xue, Q. Wang, X. Wang, W. Dong, J. Wang, and H. Zha. Guided feature selection for deep visual odometry. *CoRR*, abs/1811.09935, 2018. 4
- [10] F. Xue, X. Wang, S. Li, Q. Wang, J. Wang, and H. Zha. Beyond tracking: Selecting memory and refining poses for deep visual odometry. In *The IEEE Conference on Computer Vision and Pattern Recognition (CVPR)*, June 2019. 4
- [11] Z. Yin and J. Shi. Geonet: Unsupervised learning of dense depth, optical flow and camera pose. In *Proceedings of the IEEE Conference on Computer Vision and Pattern Recognition (CVPR)*, volume 2, 2018. 4
- [12] H. Zhan, R. Garg, C. S. Weerasekera, K. Li, H. Agarwal, and I. D. Reid. Unsupervised learning of monocular depth estimation and visual odometry with deep feature reconstruction. *CoRR*, abs/1803.03893, 2018. 4
- [13] C. Zhao, L. Sun, P. Purkait, T. Duckett, and R. Stolkin. Learning monocular visual odometry with dense 3d mapping from dense 3d flow. *Intelligent Robots and Systems (IROS), 2018 International Conference on*, 2018. 4
- [14] T. Zhou, M. Brown, N. Snavely, and D. G. Lowe. Unsupervised learning of depth and ego-motion from video. In *CVPR*, volume 2, page 7, 2017. 4
